# Supplementary material for: Understanding Stress: A Web Interface for Mental Arithmetic Tasks in a Trier Social Stress Test
Source: arXiv:2403.10356 source file (2024-03-15)
Supplement: Supplementary file 1 [file appendix.tex]

\usepackage{url} % For formatting URLs
\usepackage{hyperref} % For creating clickable links
\usepackage{enumitem} % For customizing enumerate labels
\usepackage{booktabs}
\usepackage{graphicx}
\usepackage{lscape}
\usepackage{wrapfig}

\usepackage{graphicx}
\usepackage{caption}
\usepackage{subcaption}
\usepackage{array}
\usepackage{tabularx}
\usepackage{wrapfig}
\usepackage{subcaption}

\begin{document}
\begin{figure}
    \centering
    \begin{subfigure}{0.475\textwidth}
        \includegraphics [width=\textwidth]{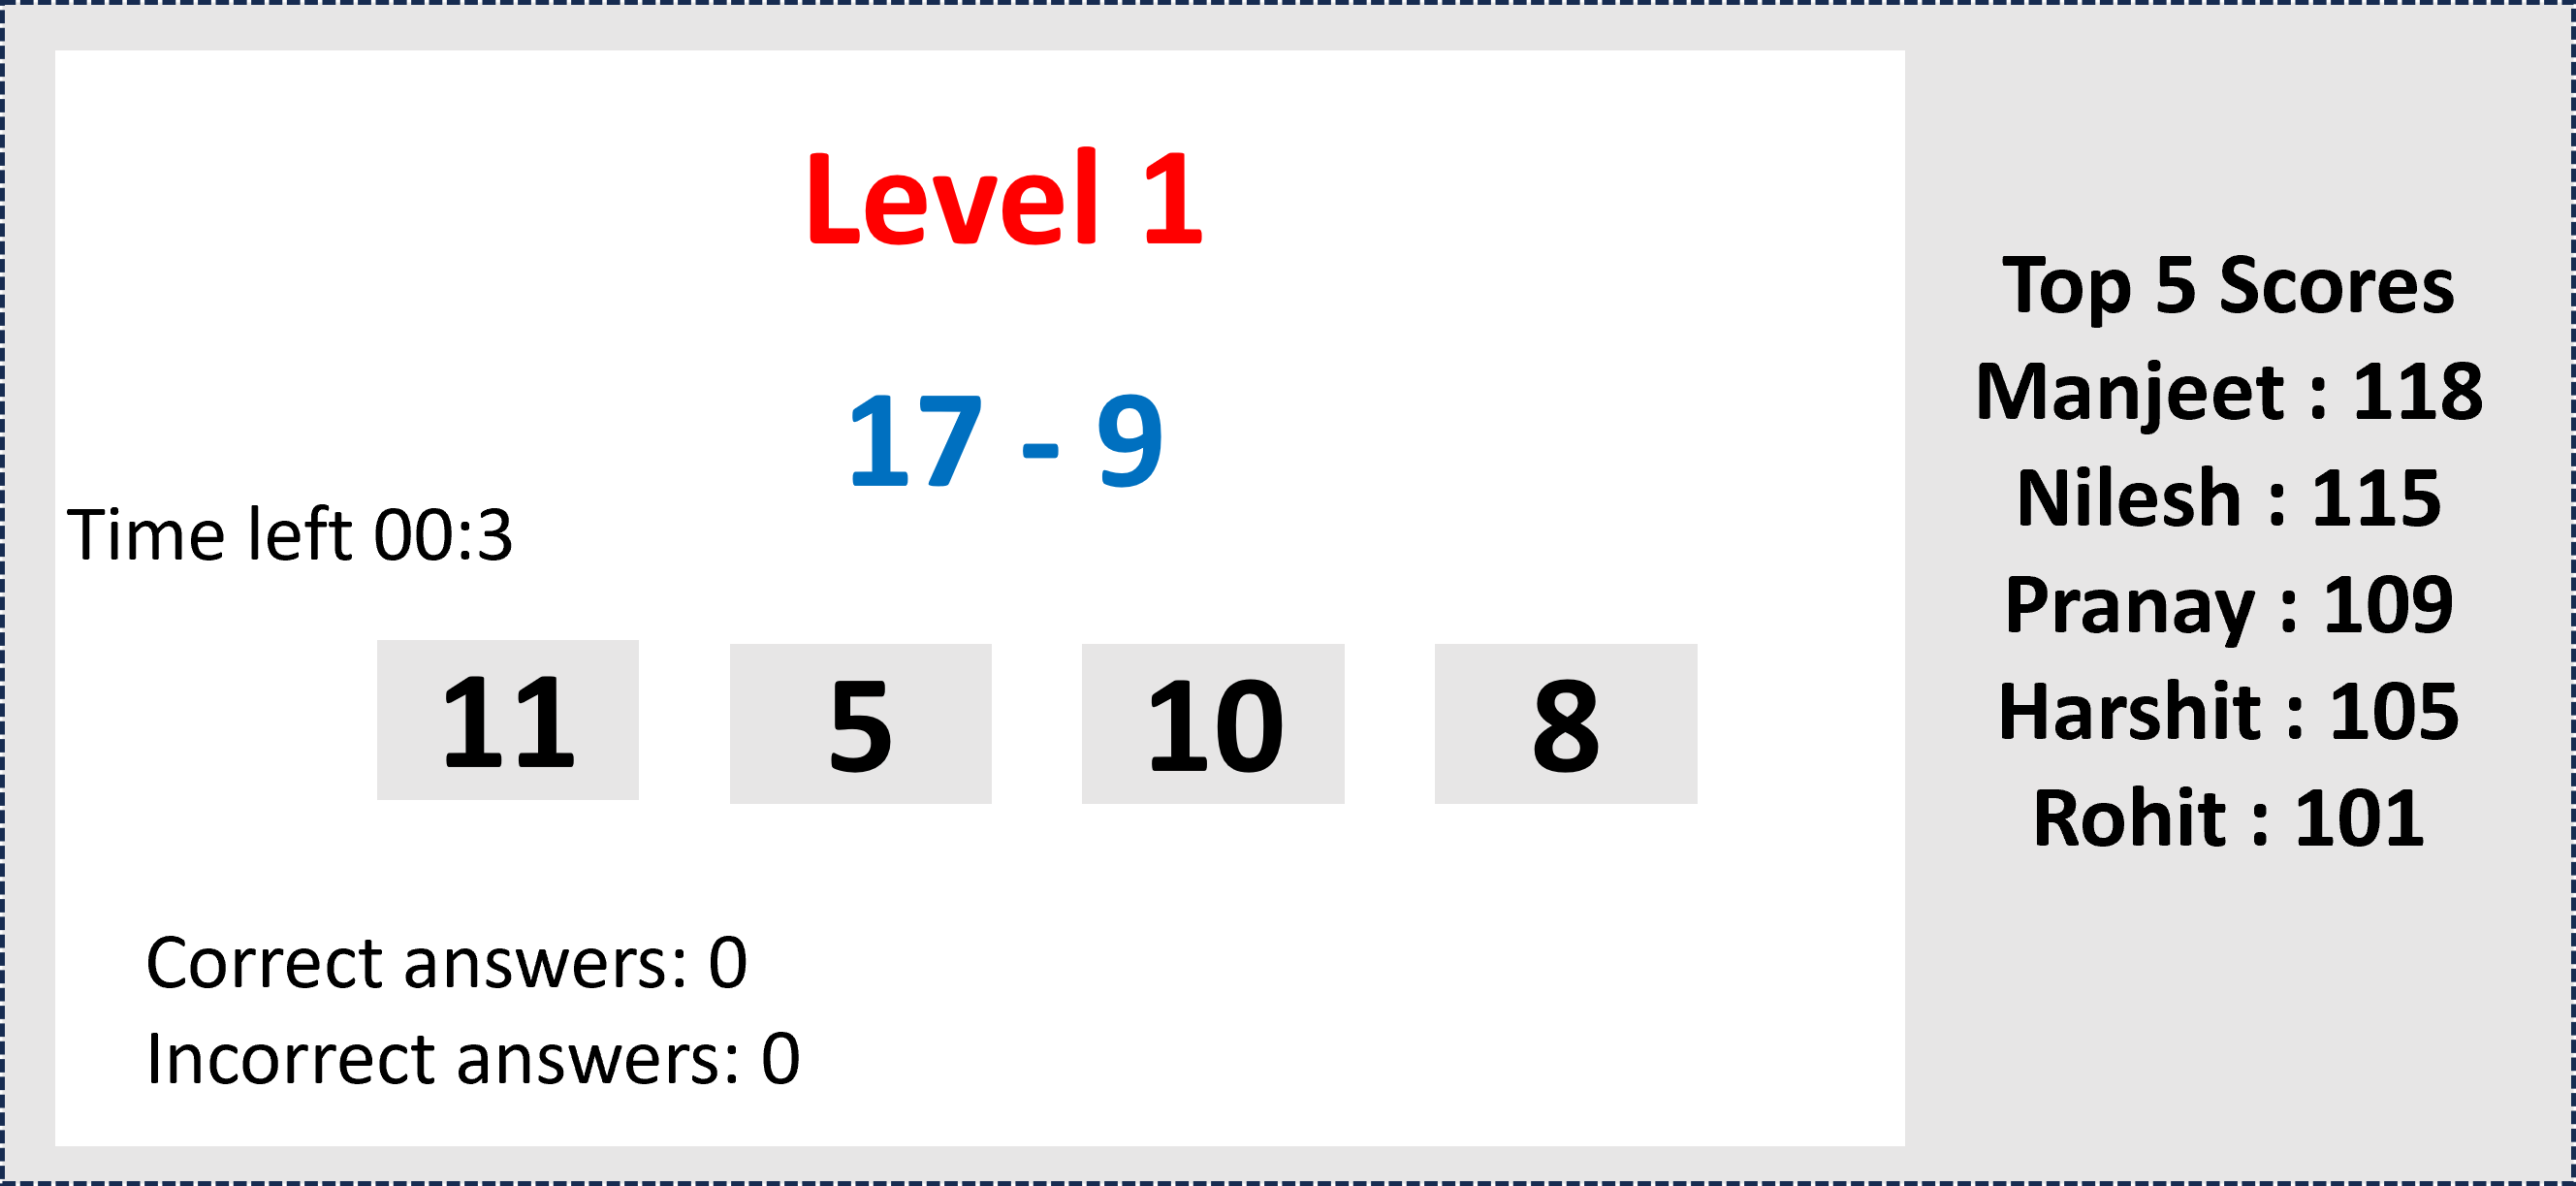}
        \caption{Level 1}
        \label{fig:Level_1}
    \end{subfigure} \hfill
        \begin{subfigure}{0.475\textwidth}
        \includegraphics [width=\textwidth]{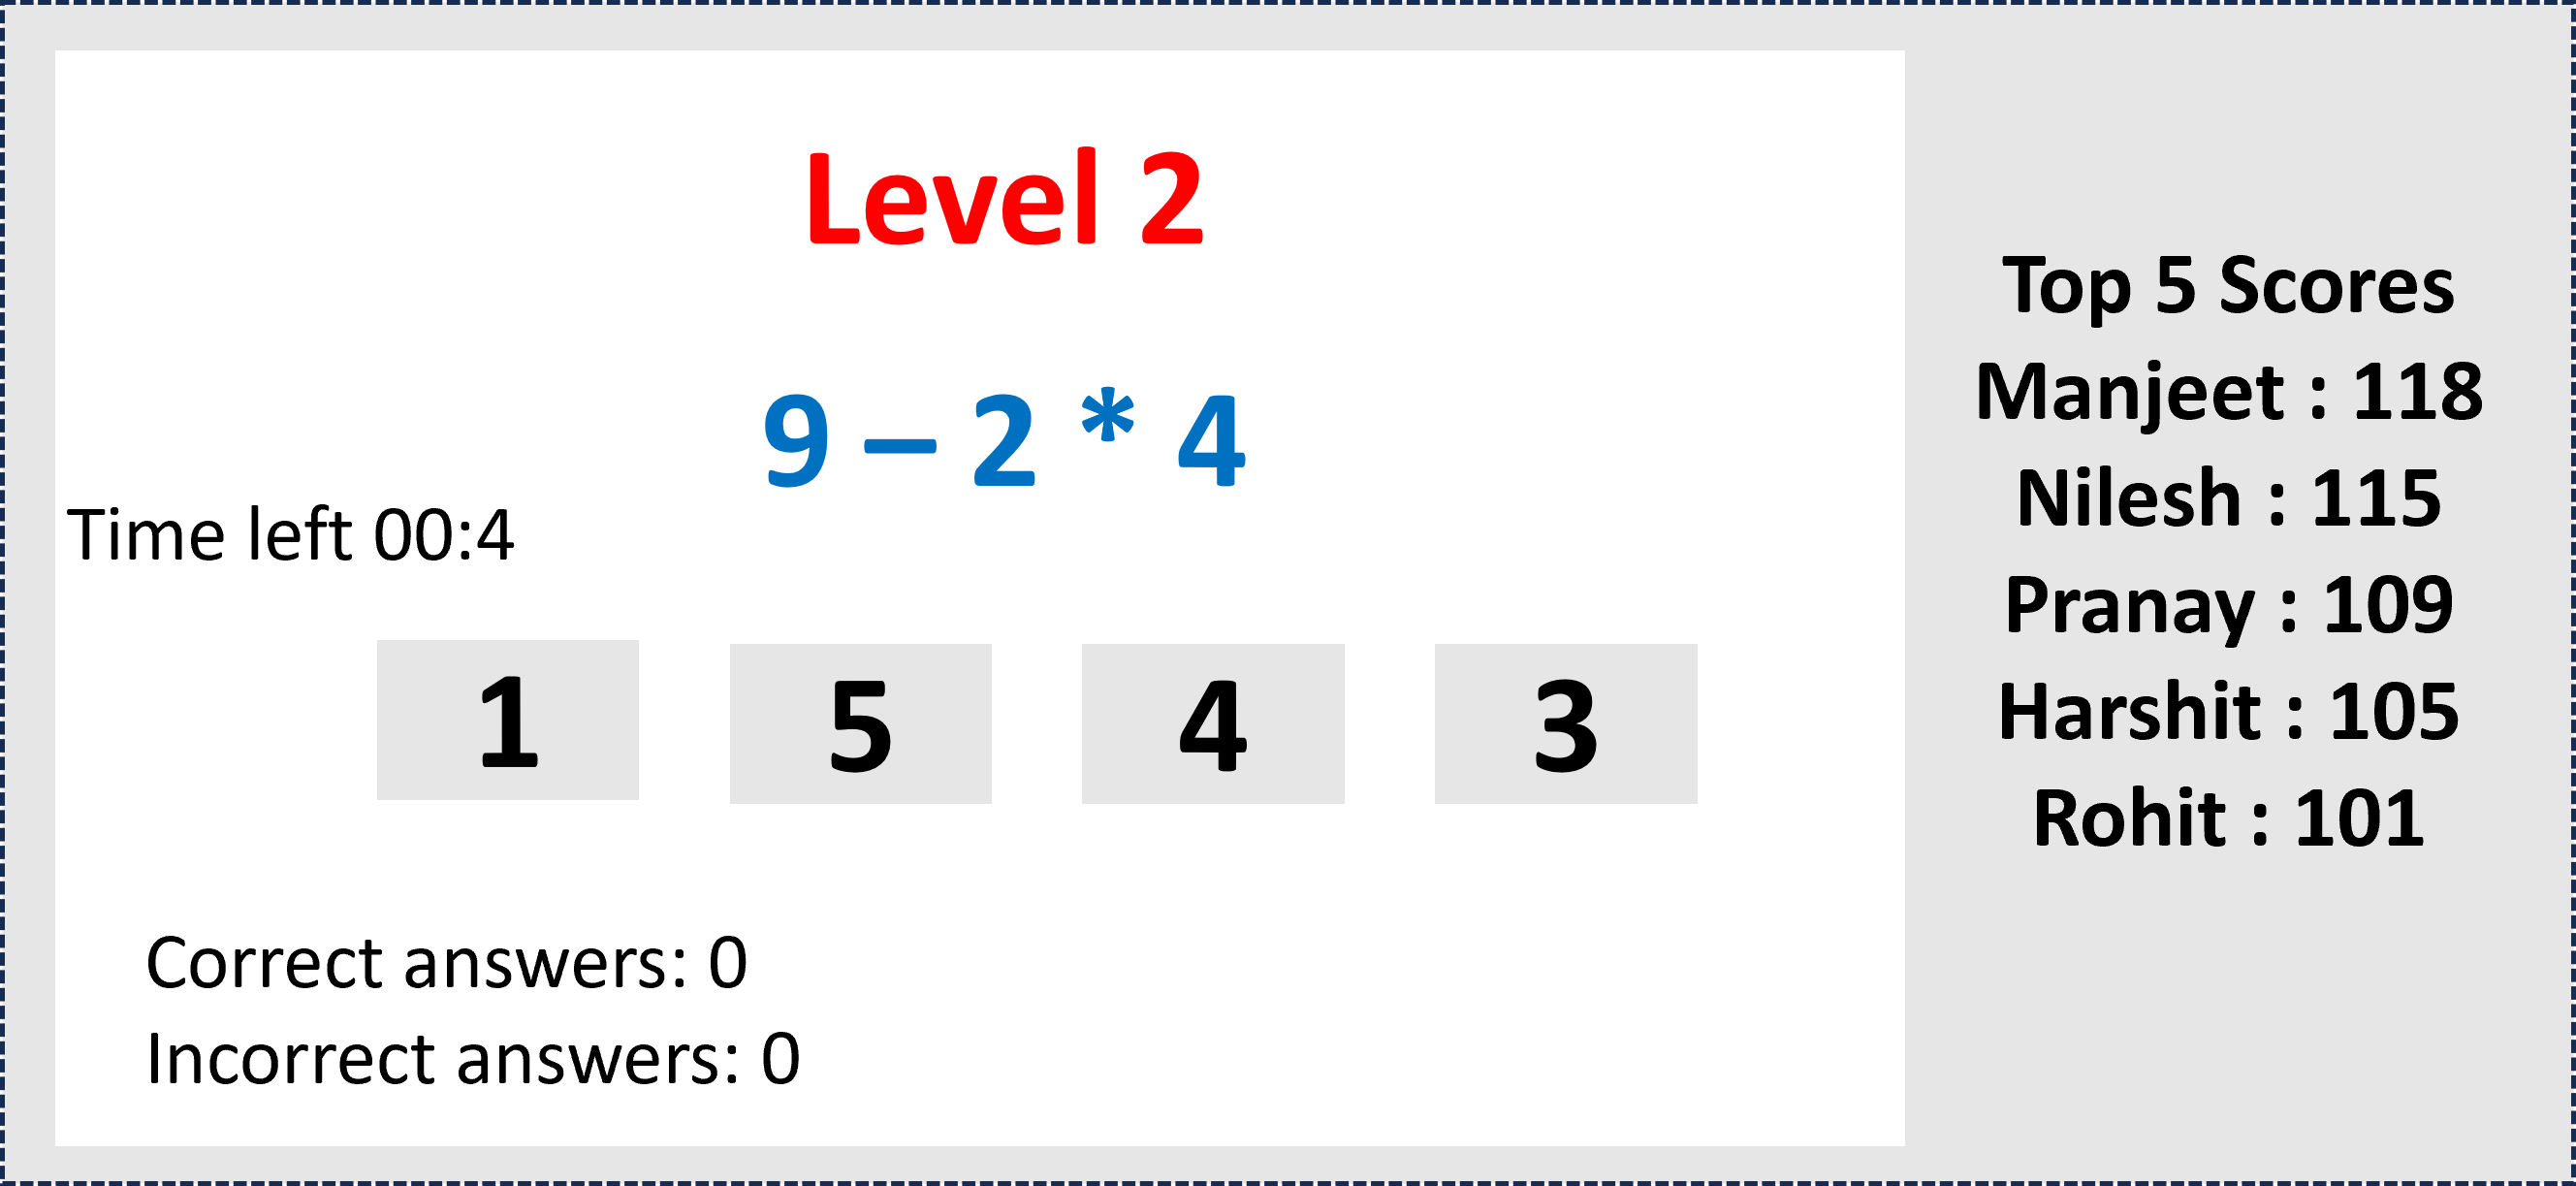}
        \caption{Level 2}
        \label{fig:Level_2}
    \end{subfigure} 
    % \medskip %<- create vertice space
    \begin{subfigure}{0.475\textwidth}
        \includegraphics [width=\textwidth]{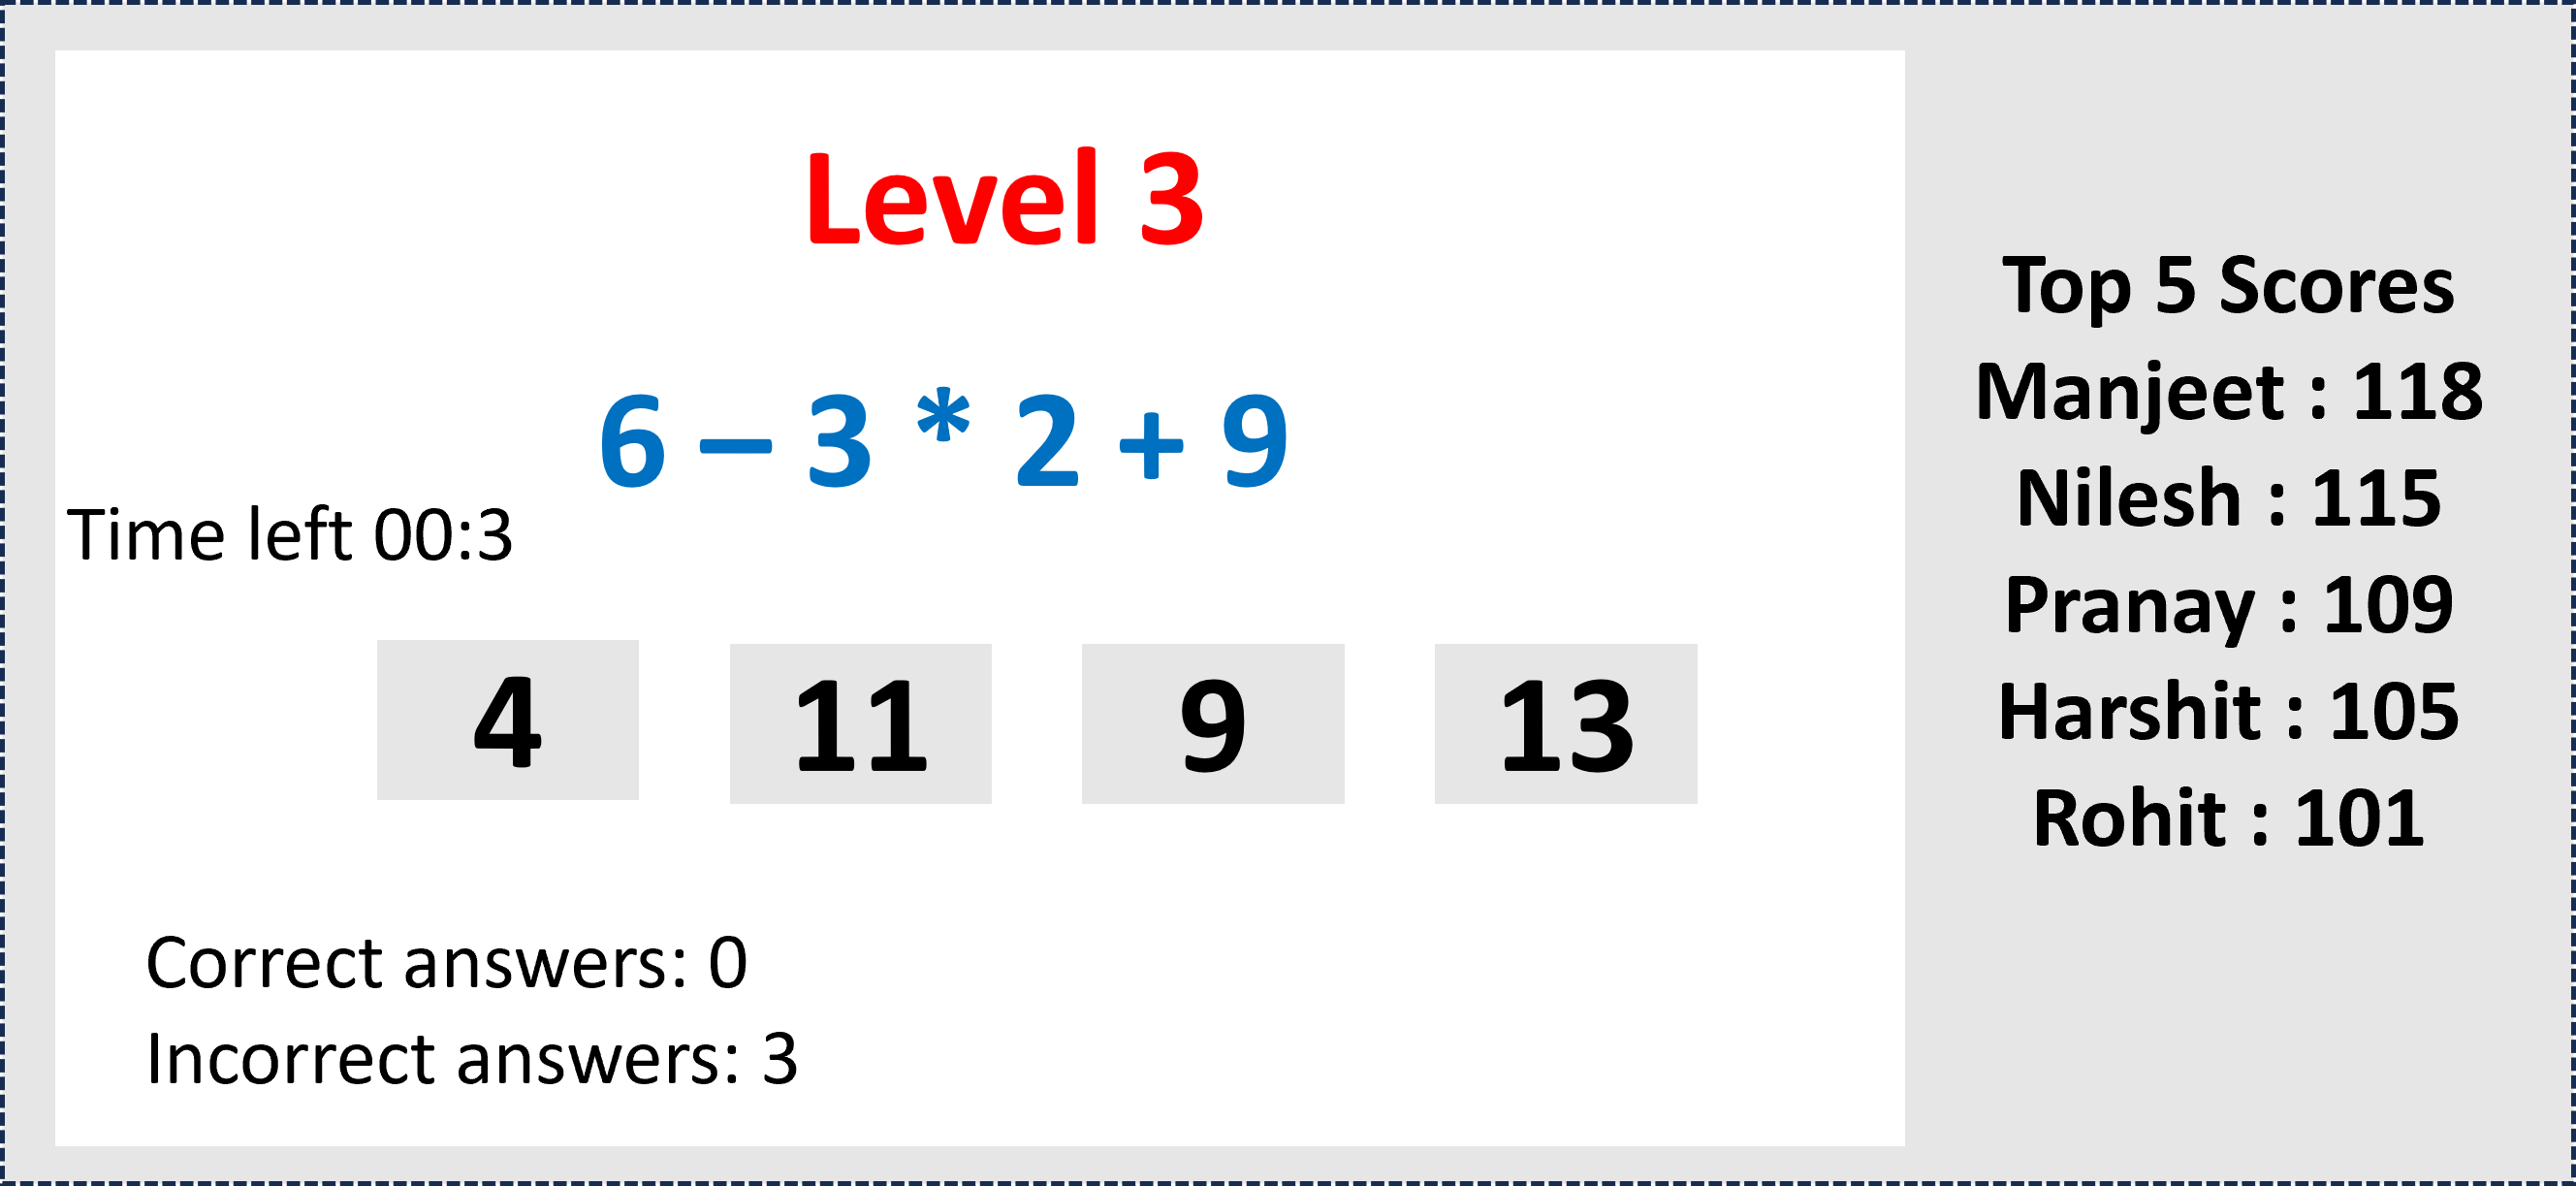}
        \caption{Level 3}
        \label{fig: Level_3}
    \end{subfigure} \hfill
    \begin{subfigure}{0.475\textwidth}
        \includegraphics [width=\textwidth]{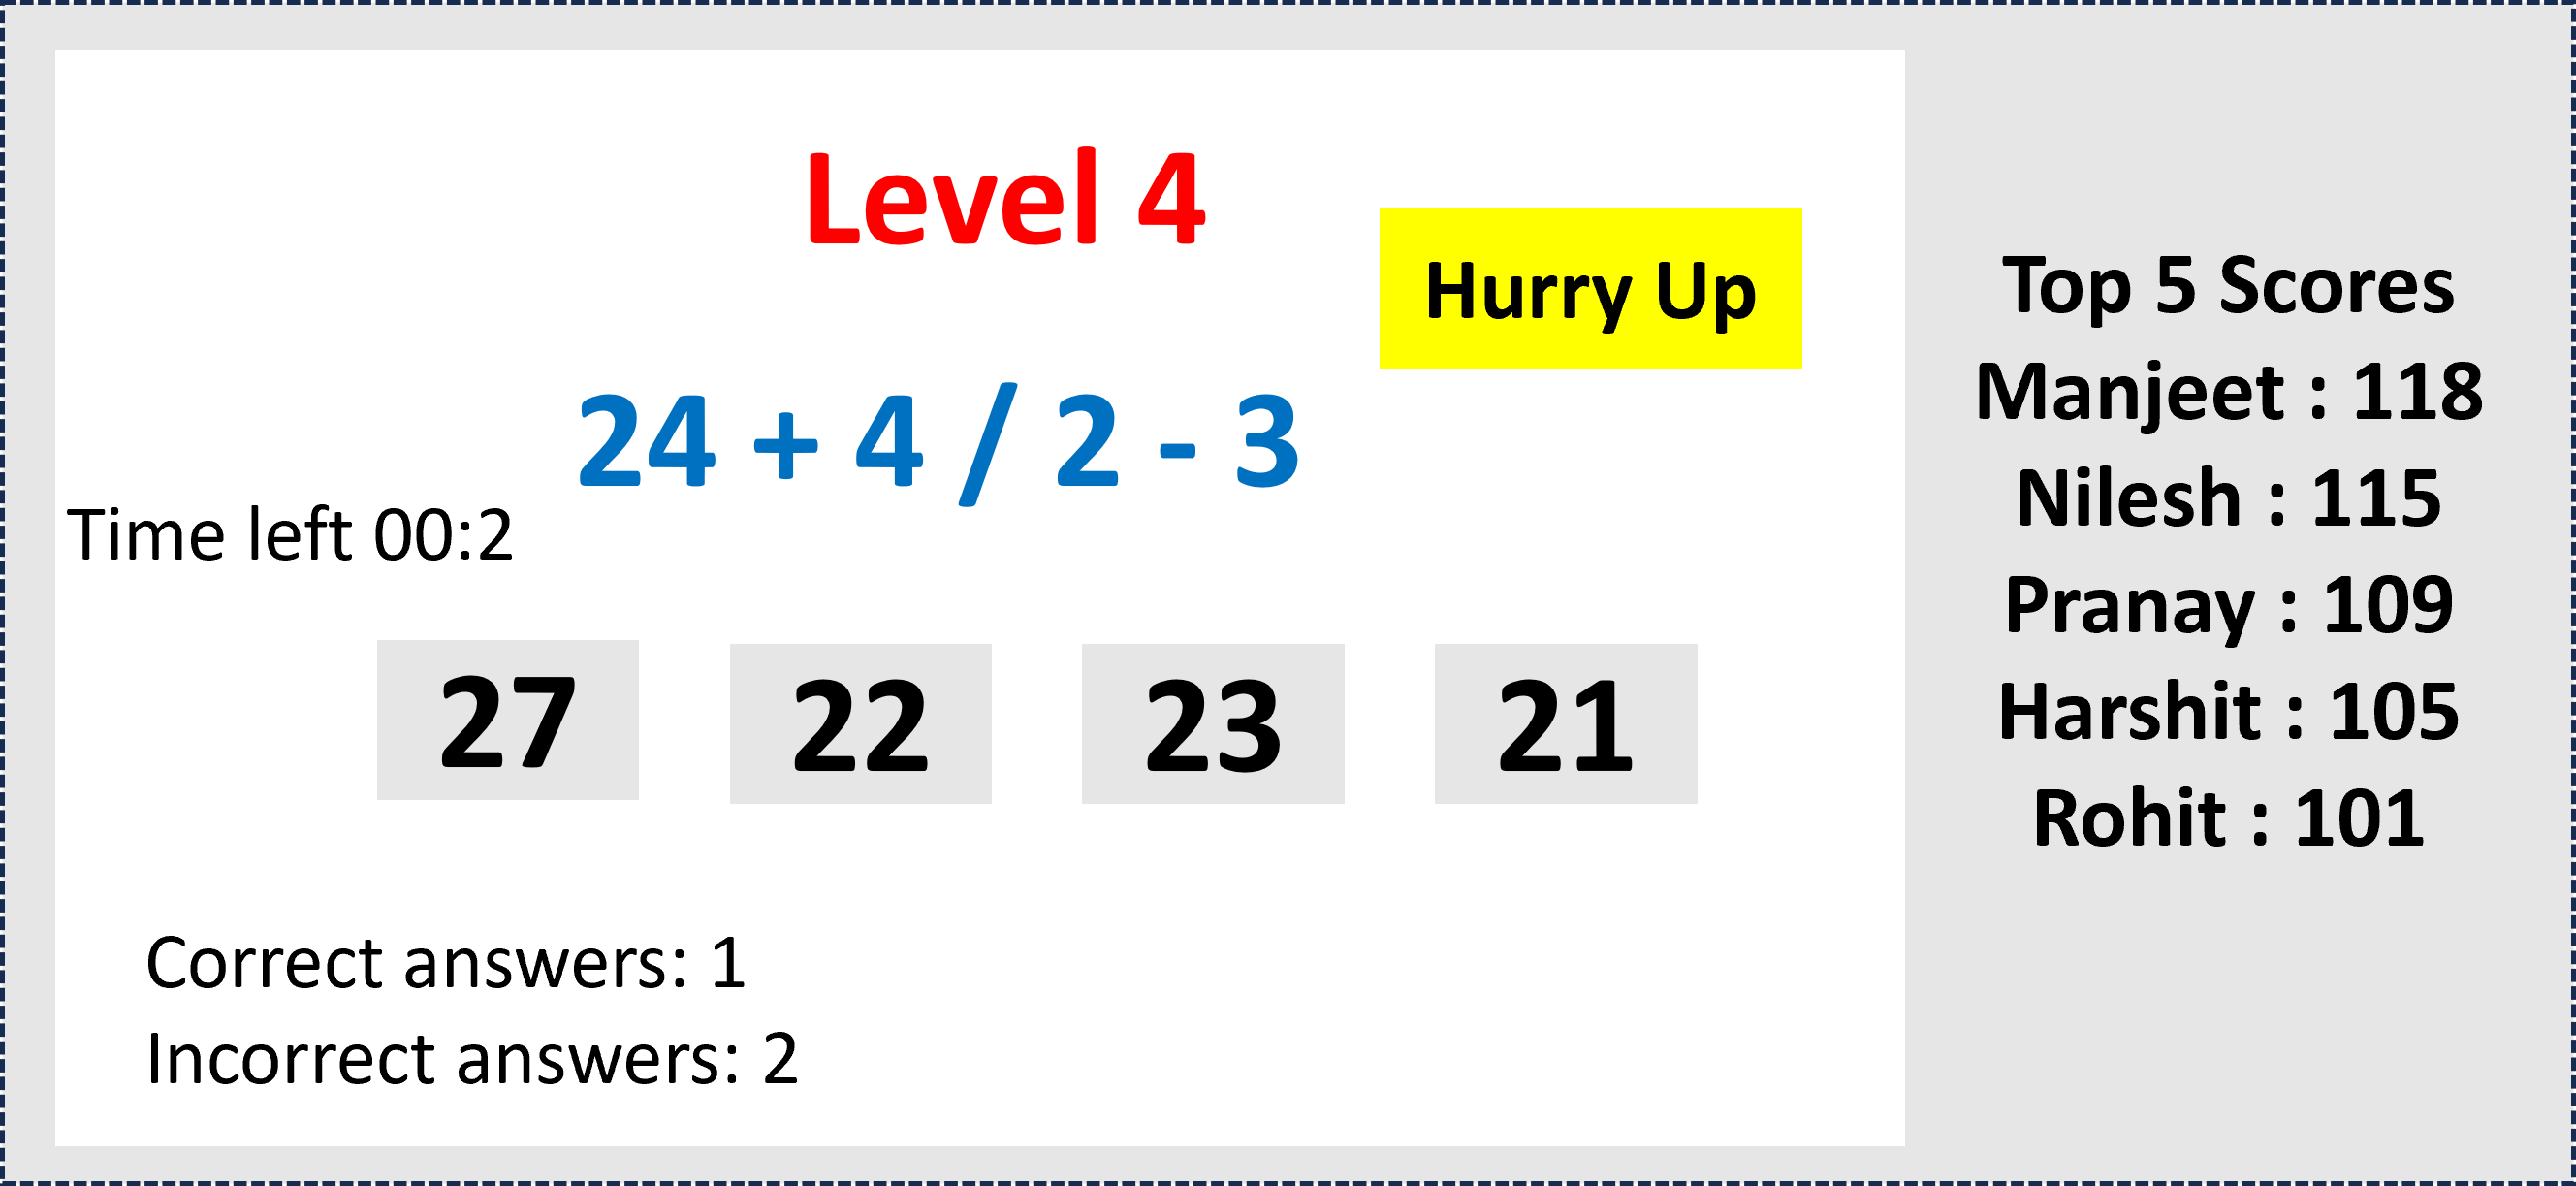}
        \caption{Level 4}
        \label{fig:Level_4}
    \end{subfigure}
    \caption{The web interface of main working area at different MAT difficulty levels}
    \label{fig:web_interface}
\end{figure}
\end{document}
